# Supplementary material for: Conditional Independence Testing for Random Objects via Generative Models
Source: arXiv:2611.28222 source file (2026-11-20)
Supplement: Supplementary file 1 [file supplement_labels.tex]

\makeatletter
\@namedef{r@app:auxiliary-lemmas}{{K}{}}
\@namedef{r@app:proof-deep-approximation}{{H}{}}
\@namedef{r@app:proof-network-covering}{{F}{}}
\@namedef{r@app:proof-paper-mds}{{E}{}}
\@namedef{r@app:proof-paper-power}{{C}{}}
\@namedef{r@app:simulation-settings}{{J}{}}
\@namedef{r@app:vector-network-rates}{{I}{}}
\@namedef{r@eq:theory-boundary-noncentral-law}{{C-46}{}}
\@namedef{r@eq:theory-lowdim-exponential-choice}{{H-2}{}}
\@namedef{r@eq:theory-lowdim-polynomial-choice}{{H-1}{}}
\@namedef{r@item:paper-mds-population}{{i}{}}
\@namedef{r@lem:appendix-mercer}{{14}{}}
\@namedef{r@lem:centered-distance-kernel}{{13}{}}
\@namedef{r@lem:paper-mds-coordinate-identities}{{9}{}}
\@namedef{r@prop:paper-network-covering}{{2}{}}
\makeatother
